# Supplementary material for: Towards near-exact solutions of molecular electronic structure: Full coupled-cluster reduction with a second-order perturbative correction
Source: arXiv:2010.01850 ancillary file (2020-11-05)
Supplement: Supplementary file 1 [file Supporting_Information.pdf]

# Supporting Information: Towards Near-Exact Solutions of Molecular Electronic Structure: Full Coupled-Cluster Reduction with a Second-Order Perturbative Correction

Enhua Xu,† Motoyuki Uejima,† and Seiichiro L. Ten-no*,†,‡

†*Graduate School of Science, Technology, and Innovation, Kobe University, Kobe 657-8501 Japan*

‡*Graduate School of System Informatics, Kobe University, Kobe 657-8501 Japan*

E-mail: tenno@garnet.kobe-u.ac.jp

# FCCR(2) equations with screenings

The CC working equation is

$$\langle\mu|\bar{H}|0\rangle = \langle\mu|\exp(-T_{\mathcal{P}})\hat{H}\exp(T_{\mathcal{P}})|0\rangle = 0. \tag{1}$$

In FCCR, this is modified using screening parameter $\theta_{\mathcal{O}}$ as

$$\begin{aligned}\langle\mu|\bar{H}|0\rangle \Rightarrow &\langle\mu|\hat{H}|0\rangle + \sum_{o}^{|\bar{t}_o|>\vartheta_{\mathcal{O}}} \langle\mu|[\hat{H},\hat{T}_o]|0\rangle \\ &+ \frac{1}{2}\sum_{o\pi}^{|\bar{t}_o\bar{t}_\pi|>\vartheta_{\mathcal{O}}} \langle\mu|[[\hat{H},\hat{T}_o],\hat{T}_\pi]|0\rangle \\ &+ \frac{1}{6}\sum_{o\pi\theta}^{|\bar{t}_o\bar{t}_\pi\bar{t}_\theta|>\vartheta_{\mathcal{O}}} \langle\mu|[[[\hat{H},\hat{T}_o],\hat{T}_\pi],\hat{T}_\theta]|0\rangle \\ &+ \frac{1}{24}\sum_{o\pi\theta\rho}^{|\bar{t}_o\bar{t}_\pi\bar{t}_\theta\bar{t}_\rho|>\vartheta_{\mathcal{O}}} \langle\mu|[[[[\hat{H},\hat{T}_o],\hat{T}_\pi],\hat{T}_\theta],\hat{T}_\rho]|0\rangle = 0,\end{aligned} \tag{2}$$

where the arrow means the screened form, and the modified amplitude takes unity when the index coincides to the bra state containing EPV terms:

$$\bar{t}_o = \begin{cases} 1 & (o = \mu) \\ t_o & (\text{otherwise}) \end{cases} \tag{3}$$

This is equivalent to the EPV form of the FCCR working equation. The non-EPV form employs the original amplitudes $t_o$ instead of $\bar{t}_o$, and can discard some important contribution of EPV by the screening.

In a similar way, the woking equation for $\hat{\Lambda}$ is

$$
\begin{aligned}
\langle 0|(1+\hat{\Lambda})[\bar{H},\hat{a}_\nu^\dagger]|0\rangle \Rightarrow \langle 0|[\hat{H},\hat{a}_\nu^\dagger]|0\rangle &+ \sum_{o}^{|t_o|>\vartheta_{\mathcal{O}}} \langle 0|[[\hat{H},\hat{T}_o],\hat{a}_\nu^\dagger]|0\rangle \\
&+ \sum_{\mu}^{|\bar{l}_\mu|>\vartheta_{\mathcal{O}}} l_\mu \langle \mu|[\hat{H},\hat{a}_\nu^\dagger]|0\rangle + \sum_{o}^{|\bar{l}_\mu \bar{t}_o|>\vartheta_{\mathcal{O}}} l_\mu \langle \mu|[[\hat{H},\hat{T}_o],\hat{a}_\nu^\dagger]|0\rangle \\
&+ \frac{1}{2}\sum_{o\pi}^{|\bar{l}_\mu \bar{t}_o \bar{t}_\pi|>\vartheta_{\mathcal{O}}} l_\mu \langle \mu|[[[\hat{H},\hat{T}_o],\hat{T}_\pi],\hat{a}_\nu^\dagger]|0\rangle \\
&+ \frac{1}{6}\sum_{o\pi\theta}^{|\bar{l}_\mu \bar{t}_o \bar{t}_\pi \bar{t}_\theta|>\vartheta_{\mathcal{O}}} l_\mu \langle \mu|[[[[\hat{H},\hat{T}_o],\hat{T}_\pi],\hat{T}_\theta],\hat{a}_\nu^\dagger]|0\rangle = 0,
\end{aligned}
\tag{4}
$$

where the modified $\hat{\Lambda}$ amplitude is unity for EPV, i.e., at least one index of $T_{\mathcal{P}}$ or $\hat{a}_\nu^\dagger$ in the commutators coincides to the bra index:

$$
\bar{l}_\mu = \begin{cases} 1 & \text{(EPV)} \\ l_\mu & \text{(otherwise)} \end{cases}
\tag{5}
$$

Using the same expressions, the $\eta_\kappa$ and $\sigma_\kappa$ objects are calculated as

$$
\begin{aligned}
\eta_\kappa =& \langle 0|(1+\hat{\Lambda})\bar{H}|\kappa\rangle \\
\Rightarrow& \langle 0|\hat{H}|\kappa\rangle + \sum_{o}^{|t_o|>\vartheta_{\mathcal{O}}} \langle 0|[\hat{H},\hat{T}_o]|\kappa\rangle \\
&+ \sum_{\mu}^{|l_\mu|>\vartheta_{\mathcal{O}}} l_\mu \langle \mu|\hat{H}|\kappa\rangle + \sum_{o}^{|\bar{l}_\mu \bar{t}_o|>\vartheta_{\mathcal{O}}} l_\mu \langle \mu|[\hat{H},\hat{T}_o]|\kappa\rangle \\
&+ \frac{1}{2}\sum_{o\pi}^{|\bar{l}_\mu \bar{t}_o \bar{t}_\pi|>\vartheta_{\mathcal{O}}} l_\mu \langle \mu|[[\hat{H},\hat{T}_o],\hat{T}_\pi]|\kappa\rangle \\
&+ \frac{1}{6}\sum_{o\pi\theta}^{|\bar{l}_\mu \bar{t}_o \bar{t}_\pi \bar{t}_\theta|>\vartheta_{\mathcal{O}}} {}_\mu \langle \mu|[[[\hat{H},\hat{T}_o],\hat{T}_\pi],\hat{T}_\theta]|\kappa\rangle \\
&+ \frac{1}{24}\sum_{o\pi\theta\rho}^{|\bar{l}_\mu \bar{t}_o \bar{t}_\pi \bar{t}_\theta \bar{t}_\rho|>\vartheta_{\mathcal{O}}} l_\mu \langle \mu|[[[[\hat{H},\hat{T}_o],\hat{T}_\pi],\hat{T}_\theta],\hat{T}_\rho]|\kappa\rangle,
\end{aligned}
\tag{6}
$$

and

$$
\begin{aligned}
\sigma_\kappa =& \langle \kappa | \bar{H} | 0 \rangle \\
\Rightarrow& \langle \kappa | \hat{H} | 0 \rangle + \sum_{o}^{|t_o| > \vartheta_{\mathcal{O}}} \langle \kappa | [\hat{H}, \hat{T}_o] | 0 \rangle \\
&+ \frac{1}{2} \sum_{o\pi}^{|t_o t_\pi| > \vartheta_{\mathcal{O}}} \langle \kappa | [[\hat{H}, \hat{T}_o], \hat{T}_\pi] | 0 \rangle \\
&+ \frac{1}{6} \sum_{o\pi\theta}^{|t_o t_\pi t_\theta| > \vartheta_{\mathcal{O}}} \langle \kappa | [[[\hat{H}, \hat{T}_o], \hat{T}_\pi], \hat{T}_\theta] | 0 \rangle \\
&+ \frac{1}{24} \sum_{o\pi\theta\rho}^{|t_o t_\pi t_\theta t_\rho| > \vartheta_{\mathcal{O}}} \langle \kappa | [[[[\hat{H}, \hat{T}_o], \hat{T}_\pi], \hat{T}_\theta], \hat{T}_\rho] | 0 \rangle .
\end{aligned}
\tag{7}
$$

# Approximations for FCCR(2')

Around the equilibrium geometry, we can use some approximations to $\{\eta_\kappa\}$ and $\{\sigma_\kappa\}$ to simplify the computation of the objects. In FCCR(2') employed for the blind test of benzene, the following approximations are made. For $\eta_\kappa$, $\hat{\Lambda}$ is approximated by $\hat{T}^\dagger_\mathcal{P}$ and $\bar{H}$ is replaced by $\hat{H}$:

$$\begin{aligned}\eta_\kappa =&\langle 0|(1+\hat{\Lambda})\bar{H}|\kappa\rangle \approx \langle 0|(1+\hat{T}^\dagger_\mathcal{P})\hat{H}|\kappa\rangle \\ \Rightarrow&\langle 0|\hat{H}|\kappa\rangle + \sum_{\mu}^{|t_\mu|>\vartheta_\mathcal{O}} t_\mu \langle \mu|\hat{H}|\kappa\rangle,\end{aligned} \tag{8}$$

and the similarity transformed Hamiltonian is terminated at the single commutator in $\sigma_\kappa$ as

$$\begin{aligned}\sigma_\kappa =&\langle \kappa|\bar{H}|0\rangle \approx \langle \kappa|\hat{H} + [\hat{H}, \hat{T}_\mathcal{P}]|0\rangle \\ \Rightarrow&\langle \kappa|\hat{H}|0\rangle + \sum_{\mu}^{|t_\mu|>\vartheta_\mathcal{O}} \langle \kappa|[\hat{H}, \hat{T}_\mu]|0\rangle.\end{aligned} \tag{9}$$

When $\mathcal{P}$ spans all singles and doubles, FCCR(2') is equivalent to CCSD(T).

# Detail of the results

All numerical results are detailed in the following.

Table 1: Detail of FCCR(2) calculation for $N_2$ in cc-pVTZ at the bond length 2.068 Bohr. The HF energy is $E_{\mathrm{HF}} = -108.9840934 E_{\mathrm{H}}$. $\Delta E_{\mathrm{RMSD}}$ is for 4 point extrapolations, and all energies are in m$E_{\mathrm{H}}$.

| $\vartheta_{\mathcal{P}}$ | $\Delta E_{\mathrm{FCCR(2)}}$ | $E^{(2)}$ | $\Delta E_{\mathrm{FCCR(EN2)}}$ | $E^{(\mathrm{EN2})}$ | $N_{\mathcal{P}}$ | $N_{\mathcal{Q}}$ |
|---|---|---|---|---|---|---|
| $5 \times 10^{-4}$ | -389.70 | -14.00 | -391.48 | -15.77 | 8,518 | $4.7 \times 10^6$ |
| $4 \times 10^{-4}$ | -389.89 | -12.06 | -391.43 | -13.60 | 10,178 | $6.4 \times 10^6$ |
| $3 \times 10^{-4}$ | -390.10 | -9.95 | -391.37 | -11.22 | 12,942 | $9.5 \times 10^6$ |
| $2 \times 10^{-4}$ | -390.29 | -7.72 | -391.26 | -8.69 | 18,787 | $1.5 \times 10^7$ |
| Extrap. (4p) | -391.02 | | -391.01 | | | |
| Extrap. (2p) | -390.95 | | -390.90 | | | |
| $\Delta E_{\mathrm{RMSD}}$ | 0.007 | | 0.013 | | | |

Table 2: Detail of FCCR(2) calculation for $N_2$ in cc-pVQZ. $E_{\mathrm{HF}} = -108.9917353 E_{\mathrm{H}}$.

| $\vartheta_{\mathcal{P}}$ | $\Delta E_{\mathrm{FCCR(2)}}$ | $E^{(2)}$ | $\Delta E_{\mathrm{FCCR(EN2)}}$ | $E^{(\mathrm{EN2})}$ | $N_{\mathcal{P}}$ | $N_{\mathcal{Q}}$ |
|---|---|---|---|---|---|---|
| $5 \times 10^{-4}$ | -411.66 | -27.13 | -413.91 | -29.37 | 12,580 | $2.3 \times 10^7$ |
| $4 \times 10^{-4}$ | -412.16 | -21.99 | -414.04 | -23.87 | 15,914 | $3.0 \times 10^7$ |
| $3 \times 10^{-4}$ | -412.61 | -16.91 | -414.11 | -18.40 | 21,469 | $4.6 \times 10^7$ |
| $2 \times 10^{-4}$ | -412.98 | -12.54 | -414.13 | -13.69 | 31,253 | $7.8 \times 10^7$ |
| Extrap. (4p) | -414.14 | | -414.35 | | | |
| Extrap. (2p) | -414.06 | | -414.20 | | | |
| $\Delta E_{\mathrm{RMSD}}$ | 0.017 | | 0.026 | | | |

Table 3: Detail of FCCR(2) calculation for $N_2$ in cc-pV5Z. $E_{\text{HF}} = -108.9934198 E_{\text{H}}$.

| $\vartheta_{\mathcal{P}}$ | $\Delta E_{\text{FCCR(2)}}$ | $E^{(2)}$ | $\Delta E_{\text{FCCR(EN2)}}$ | $E^{(\text{EN2})}$ | $N_{\mathcal{P}}$ | $N_{\mathcal{Q}}$ |
|---|---|---|---|---|---|---|
| $5 \times 10^{-4}$ | -419.38 | -38.50 | -421.83 | -40.95 | 15,856 | $7.4 \times 10^7$ |
| $4 \times 10^{-4}$ | -419.87 | -32.57 | -421.95 | -34.64 | 19,885 | $9.9 \times 10^7$ |
| $3 \times 10^{-4}$ | -420.35 | -25.94 | -422.02 | -27.61 | 26,810 | $1.5 \times 10^8$ |
| $2 \times 10^{-4}$ | -420.82 | -18.75 | -422.07 | -20.00 | 40,919 | $2.6 \times 10^8$ |
| Extrap. (4p) | -422.20 | | -422.32 | | | |
| Extrap. (2p) | -422.04 | | -422.20 | | | |
| $\Delta E_{\text{RMSD}}$ | 0.027 | | 0.020 | | | |

Table 4: Detail of FCCR(2) calculation for benzene in the equilibrium geometry in cc-pVDZ. $E_{\text{HF}} = -230.7218191 E_{\text{H}}$.

| $\vartheta_{\mathcal{P}}$ | $\Delta E_{\text{FCCR(2)}}$ | $E^{(2)}$ | $\Delta E_{\text{FCCR(EN2)}}$ | $E^{(\text{EN2})}$ | $N_{\mathcal{P}}$ | $N_{\mathcal{Q}}$ |
|---|---|---|---|---|---|---|
| $5 \times 10^{-4}$ | -849.04 | -81.09 | -845.93 | -77.97 | 109,860 | $2.2 \times 10^8$ |
| $4 \times 10^{-4}$ | -852.25 | -62.36 | -849.96 | -60.06 | 137,421 | $2.6 \times 10^8$ |
| $3 \times 10^{-4}$ | -854.93 | -46.71 | -853.40 | -45.18 | 174,914 | $3.7 \times 10^8$ |
| $2 \times 10^{-4}$ | -856.83 | -35.10 | -855.89 | -34.16 | 229,842 | $6.4 \times 10^8$ |
| Extrap. (4p) | -862.82 | | -863.67 | | | |
| Extrap. (2p) | -862.58 | | -863.61 | | | |
| $\Delta E_{\text{RMSD}}$ | 0.027 | | 0.021 | | | |

Table 5: Detail of FCCR(2) calculation for benzene in the stretched geometry. $E_{\text{HF}} = -229.0988737 E_{\text{H}}$.

| $\vartheta_{\mathcal{P}}$ | $\Delta E_{\text{FCCR(2)}}$ | $E^{(2)}$ | $\Delta E_{\text{FCCR(EN2)}}$ | $E^{(\text{EN2})}$ | $N_{\mathcal{P}}$ | $N_{\mathcal{Q}}$ |
|---|---|---|---|---|---|---|
| $5 \times 10^{-4}$ | -1,229.92 | -119.06 | -1,210.61 | -99.75 | 136,285 | $1.3 \times 10^9$ |
| $4 \times 10^{-4}$ | -1,232.78 | -104.36 | -1,215.85 | -87.42 | 178,333 | $1.8 \times 10^9$ |
| $3 \times 10^{-4}$ | -1,235.60 | -89.52 | -1,221.15 | -75.06 | 249,952 | $3.0 \times 10^9$ |
| $2 \times 10^{-4}$ | -1,238.63 | -73.55 | -1,226.98 | -61.91 | 411,628 | $5.9 \times 10^9$ |
| Extrap. (4p) | -1,252.70 | | -1,253.69 | | | |
| Extrap. (2p) | -1,252.57 | | -1,254.46 | | | |
| $\Delta E_{\text{RMSD}}$ | 0.020 | | 0.063 | | | |

Table 6: FCCR(2) calculation details for the peroxo isomer of $[Cu_2O_2(NH_3)_2]^{2+}$. $E_{\text{HF}} = -3539.3565429 E_{\text{H}}$.

| $\vartheta_{\mathcal{P}}$ | $\Delta E_{\text{FCCR(2)}}$ | $E^{(2)}$ | $\Delta E_{\text{FCCR(EN2)}}$ | $E^{(\text{EN2})}$ | $N_{\mathcal{P}}$ | $N_{\mathcal{Q}}$ |
|---|---|---|---|---|---|---|
| $5 \times 10^{-4}$ | -1,805.39 | -312.50 | -1,764.39 | -271.50 | 205,548 | $1.3 \times 10^{10}$ |
| $4 \times 10^{-4}$ | -1,810.90 | -252.46 | -1,776.51 | -218.06 | 278,616 | $1.6 \times 10^{10}$ |
| $3 \times 10^{-4}$ | -1,816.05 | -194.63 | -1,789.01 | -167.60 | 397,897 | $2.1 \times 10^{10}$ |
| $2 \times 10^{-4}$ | -1,820.63 | -138.23 | -1,801.36 | -118.97 | 625,816 | $3.5 \times 10^{10}$ |
| Extrap. (4p) | -1,832.90 | | -1,829.94 | | | |
| Extrap. (2p) | -1,831.85 | | -1,831.58 | | | |
| $\Delta E_{\text{RMSD}}$ | 0.155 | | 0.362 | | | |

Table 7: Detail of FCCR(2) calculation for the bis($\mu$-oxo) isomer of $[Cu_2O_2(NH_3)_2]^{2+}$. $E_{\mathrm{HF}} = -3539.2523877 E_{\mathrm{H}}$. The resulting inverconversion energies of FCCR(EN2) and FCCR(EN2)-Ex are 27.32 and 24.35 kcal/mol, respectively.

| $\vartheta_{\mathcal{P}}$ | $\Delta E_{\mathrm{FCCR(2)}}$ | $E^{(2)}$ | $\Delta E_{\mathrm{FCCR(EN2)}}$ | $E^{(\mathrm{EN2})}$ | $N_{\mathcal{P}}$ | $N_{\mathcal{Q}}$ |
|---|---|---|---|---|---|---|
| $5 \times 10^{-4}$ | -1,865.80 | -317.24 | -1,822.50 | -273.95 | 203,935 | $1.4 \times 10^{10}$ |
| $4 \times 10^{-4}$ | -1,871.58 | -259.50 | -1,835.15 | -223.07 | 277,596 | $1.8 \times 10^{10}$ |
| $3 \times 10^{-4}$ | -1,877.42 | -202.65 | -1,848.61 | -173.83 | 400,920 | $2.5 \times 10^{10}$ |
| $2 \times 10^{-4}$ | -1,882.74 | -146.62 | -1,861.99 | -125.87 | 643,310 | $4.4 \times 10^{10}$ |
| Extrap. (4p) | -1,897.44 | | -1,895.28 | | | |
| Extrap. (2p) | -1,896.63 | | -1,897.10 | | | |
| $\Delta E_{\mathrm{RMSD}}$ | 0.100 | | 0.393 | | | |
